# Supplementary material for: Bridging Functional Correctness and Runtime Efficiency Gaps in LLM-Based Code Translation
Source: arXiv:2606.17683 source file (2026-06-16)
Supplement: Supplementary file 2 [file appendix_llm.tex]

\section{The Use of Large Language Models (LLMs)}
During the preparation of this paper, LLMs were used as an auxiliary tool for language refinement and formatting.
Specifically, GPT-based models were employed to enhance writing clarity, improve grammatical accuracy, and generate alternative phrasings for certain sentences.
However, LLMs played no role in generating the research ideas, methodology, experimental design, or results.
All conceptual contributions, technical developments, and data analyses were carried out by the authors.
The final content was thoroughly verified and revised by the authors, who take full responsibility for the correctness and integrity of this work.
